# Supplementary material for: Search for Boosted Dark Matter Interacting With Electrons in Super-Kamiokande
Source: arXiv:1711.05278 source file (2018-05-31)
Supplement: Supplementary file 1 [file Supplemental.pdf]

# Supplemental Material
# Search for Boosted Dark Matter Interacting With Electrons in Super-Kamiokande

C. Kachulis,[4] K. Abe,[1,38] C. Bronner,[1] Y. Hayato,[1,38] M. Ikeda,[1] K. Iyogi,[1] J. Kameda,[1,38] Y. Kato,[1] Y. Kishimoto,[1,38] Ll. Marti,[1] M. Miura,[1,38] S. Moriyama,[1,38] M. Nakahata,[1,38] Y. Nakano,[1] S. Nakayama,[1,38] Y. Okajima,[1] A. Orii,[1] G. Pronost,[1] H. Sekiya,[1,38] M. Shiozawa,[1,38] Y. Sonoda,[1] A. Takeda,[1,38] A. Takenaka,[1] H. Tanaka,[1] S. Tasaka,[1] T. Tomura,[1,38] R. Akutsu,[2] T. Kajita,[2,38] K. Kaneyuki,[2,38,*] Y. Nishimura,[2] K. Okumura,[2,38] K. M. Tsui,[2] L. Labarga,[3] P. Fernandez,[3] F. d. M. Blaszczyk,[4] J. Gustafson,[4] E. Kearns,[4,38] J. L. Raaf,[4] J. L. Stone,[4,38] L. R. Sulak,[4] S. Berkman,[5] S. Tobayama,[5] M. Goldhaber,[6,*] M. Elnimr,[7] W. R. Kropp,[7] S. Mine,[7] S. Locke,[7] P. Weatherly,[7] M. B. Smy,[7,38] H. W. Sobel,[7,38] V. Takhistov,[7,†] K. S. Ganezer,[8] J. Hill,[8] J. Y. Kim,[9] I. T. Lim,[9] R. G. Park,[9] A. Himmel,[10] Z. Li,[10] E. O'Sullivan,[10] K. Scholberg,[10,38] C. W. Walter,[10,38] T. Ishizuka,[11] T. Nakamura,[12] J. S. Jang,[13] K. Choi,[14] J. G. Learned,[14] S. Matsuno,[14] S. N. Smith,[14] J. Amey,[15] R. P. Litchfield,[15] W. Y. Ma,[15] Y. Uchida,[15] M. O. Wascko,[15] S. Cao,[16] M. Friend,[16] T. Hasegawa,[16] T. Ishida,[16] T. Ishii,[16] T. Kobayashi,[16] T. Nakadaira,[16] K. Nakamura,[16,38] Y. Oyama,[16] K. Sakashita,[16] T. Sekiguchi,[16] T. Tsukamoto,[16] KE. Abe,[17] M. Hasegawa,[17] A. T. Suzuki,[17] Y. Takeuchi,[17,38] T. Yano,[17] T. Hayashino,[18] T. Hiraki,[18] S. Hirota,[18] K. Huang,[18] M. Jiang,[18] KE. Nakamura,[18] T. Nakaya,[18,38] B. Quilain,[18] N. D. Patel,[18] R. A. Wendell,[18,38] L. H. V. Anthony,[19] N. McCauley,[19] A. Pritchard,[19] Y. Fukuda,[20] Y. Itow,[21,22] M. Murase,[21] F. Muto,[21] P. Mijakowski,[23] K. Frankiewicz,[23] C. K. Jung,[24] X. Li,[24] J. L. Palomino,[24] G. Santucci,[24] C. Vilela,[24] M. J. Wilking,[24] C. Yanagisawa,[24,‡] S. Ito,[25] D. Fukuda,[25] H. Ishino,[25] A. Kibayashi,[25] Y. Koshio,[25,38] H. Nagata,[25] M. Sakuda,[25] C. Xu,[25] Y. Kuno,[26] D. Wark,[27,33] F. Di Lodovico,[28] B. Richards,[28] R. Tacik,[29,42] S. B. Kim,[30] A. Cole,[31] L. Thompson,[31] H. Okazawa,[32] Y. Choi,[34] K. Ito,[35] K. Nishijima,[35] M. Koshiba,[36] Y. Totsuka,[36,*] Y. Suda,[37] M. Yokoyama,[37,38] R. G. Calland,[38] M. Hartz,[38] K. Martens,[38] C. Simpson,[38,27] Y. Suzuki,[38] M. R. Vagins,[38,7] D. Hamabe,[39] M. Kuze,[39] T. Yoshida,[39] M. Ishitsuka,[40] J. F. Martin,[41] C. M. Nantais,[41] H. A. Tanaka,[41] A. Konaka,[42] S. Chen,[43] L. Wan,[43] Y. Zhang,[43] R. J. Wilkes,[44] and A. Minamino[45]

(The Super-Kamiokande Collaboration)

[1]*Kamioka Observatory, Institute for Cosmic Ray Research, University of Tokyo, Kamioka, Gifu 506-1205, Japan*
[2]*Research Center for Cosmic Neutrinos, Institute for Cosmic Ray Research, University of Tokyo, Kashiwa, Chiba 277-8582, Japan*
[3]*Department of Theoretical Physics, University Autonoma Madrid, 28049 Madrid, Spain*
[4]*Department of Physics, Boston University, Boston, MA 02215, USA*
[5]*Department of Physics and Astronomy, University of British Columbia, Vancouver, BC, V6T1Z4, Canada*
[6]*Physics Department, Brookhaven National Laboratory, Upton, NY 11973, USA*
[7]*Department of Physics and Astronomy, University of California, Irvine, Irvine, CA 92697-4575, USA*
[8]*Department of Physics, California State University, Dominguez Hills, Carson, CA 90747, USA*
[9]*Department of Physics, Chonnam National University, Kwangju 500-757, Korea*
[10]*Department of Physics, Duke University, Durham NC 27708, USA*
[11]*Junior College, Fukuoka Institute of Technology, Fukuoka, Fukuoka 811-0295, Japan*
[12]*Department of Physics, Gifu University, Gifu, Gifu 501-1193, Japan*
[13]*GIST College, Gwangju Institute of Science and Technology, Gwangju 500-712, Korea*
[14]*Department of Physics and Astronomy, University of Hawaii, Honolulu, HI 96822, USA*
[15]*Department of Physics, Imperial College London , London, SW7 2AZ, United Kingdom*
[16]*High Energy Accelerator Research Organization (KEK), Tsukuba, Ibaraki 305-0801, Japan*
[17]*Department of Physics, Kobe University, Kobe, Hyogo 657-8501, Japan*
[18]*Department of Physics, Kyoto University, Kyoto, Kyoto 606-8502, Japan*
[19]*Department of Physics, University of Liverpool, Liverpool, L69 7ZE, United Kingdom*
[20]*Department of Physics, Miyagi University of Education, Sendai, Miyagi 980-0845, Japan*
[21]*Institute for Space-Earth Enviromental Research, Nagoya University, Nagoya, Aichi 464-8602, Japan*
[22]*Kobayashi-Maskawa Institute for the Origin of Particles and the Universe, Nagoya University, Nagoya, Aichi 464-8602, Japan*
[23]*National Centre For Nuclear Research, 00-681 Warsaw, Poland*
[24]*Department of Physics and Astronomy, State University of New York at Stony Brook, NY 11794-3800, USA*
[25]*Department of Physics, Okayama University, Okayama, Okayama 700-8530, Japan*
[26]*Department of Physics, Osaka University, Toyonaka, Osaka 560-0043, Japan*
[27]*Department of Physics, Oxford University, Oxford, OX1 3PU, United Kingdom*
[28]*School of Physics and Astronomy, Queen Mary University of London, London, E1 4NS, United Kingdom*
[29]*Department of Physics, University of Regina, 3737 Wascana Parkway, Regina, SK, S4SOA2, Canada*
[30]*Department of Physics, Seoul National University, Seoul 151-742, Korea*
[31]*Department of Physics and Astronomy, University of Sheffield, S10 2TN, Sheffield, United Kingdom*

[32] *Department of Informatics in Social Welfare, Shizuoka University of Welfare, Yaizu, Shizuoka, 425-8611, Japan*
[33] *STFC, Rutherford Appleton Laboratory, Harwell Oxford, and Daresbury Laboratory, Warrington, OX11 0QX, United Kingdom*
[34] *Department of Physics, Sungkyunkwan University, Suwon 440-746, Korea*
[35] *Department of Physics, Tokai University, Hiratsuka, Kanagawa 259-1292, Japan*
[36] *The University of Tokyo, Bunkyo, Tokyo 113-0033, Japan*
[37] *Department of Physics, University of Tokyo, Bunkyo, Tokyo 113-0033, Japan*
[38] *Kavli Institute for the Physics and Mathematics of the Universe (WPI), The University of Tokyo Institutes for Advanced Study, University of Tokyo, Kashiwa, Chiba 277-8583, Japan*
[39] *Department of Physics,Tokyo Institute of Technology, Meguro, Tokyo 152-8551, Japan*
[40] *Department of Physics, Faculty of Science and Technology, Tokyo University of Science, Noda, Chiba 278-8510, Japan*
[41] *Department of Physics, University of Toronto, ON, M5S 1A7, Canada*
[42] *TRIUMF, 4004 Wesbrook Mall, Vancouver, BC, V6T2A3, Canada*
[43] *Department of Engineering Physics, Tsinghua University, Beijing, 100084, China*
[44] *Department of Physics, University of Washington, Seattle, WA 98195-1560, USA*
[45] *Faculty of Engineering, Yokohama National University, Yokohama, 240-8501, Japan*

(Dated: March 23, 2018)

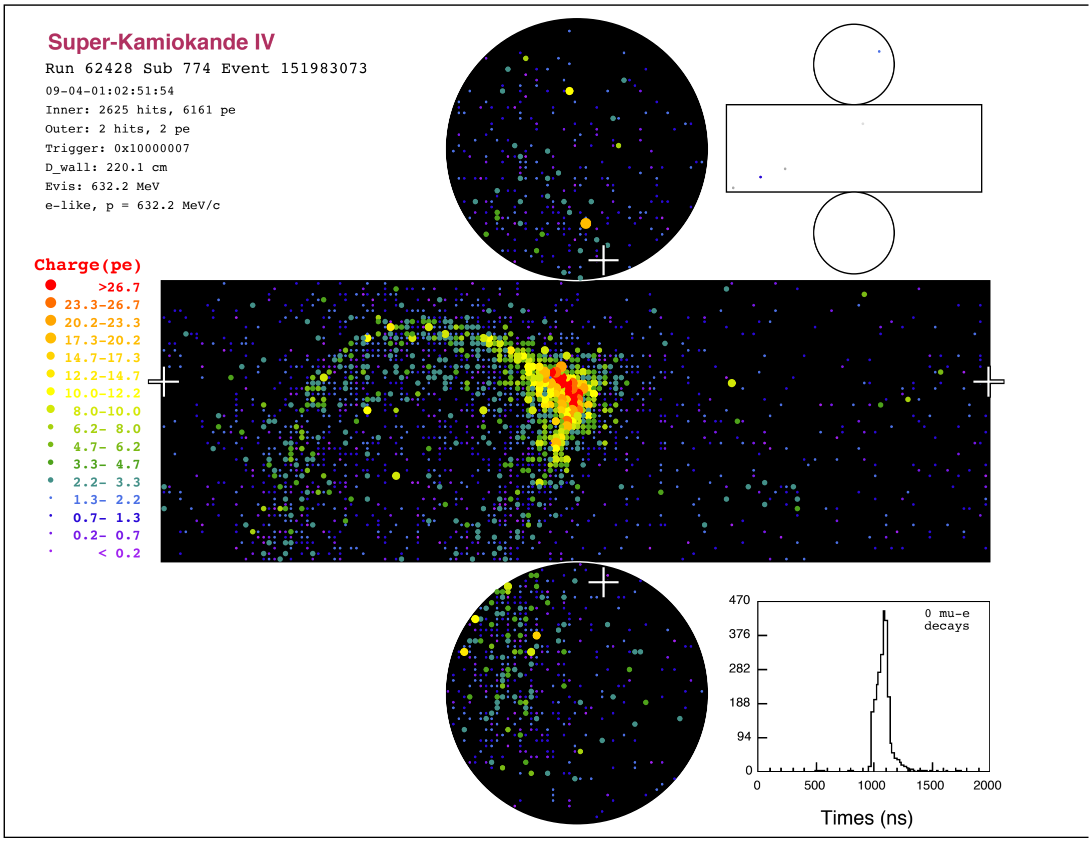


FIG. 1. An example data event passing all analysis cuts with visible energy of 632 MeV. Note the charge scale is different from those in Figs. 2 and 3.

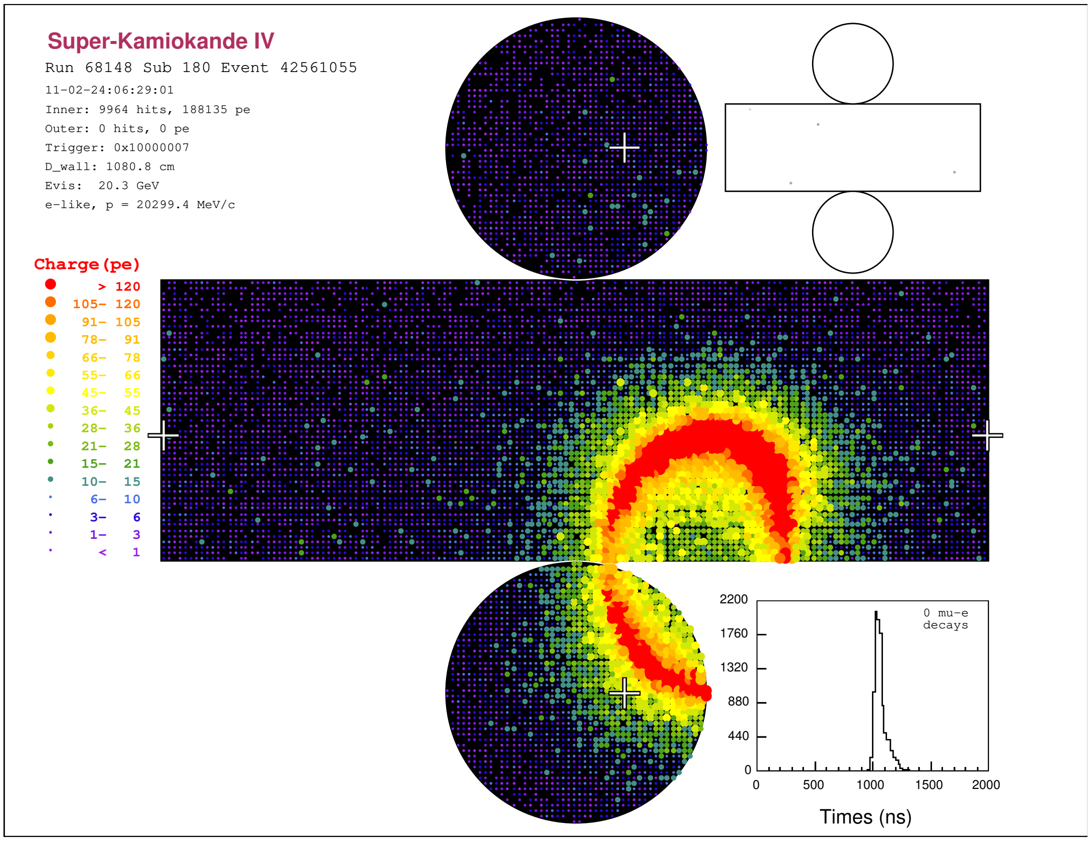


FIG. 2. An example data event passing all analysis cuts with visible energy of 20.3 GeV. Note the charge scale is different from those in Figs. 1 and 3.

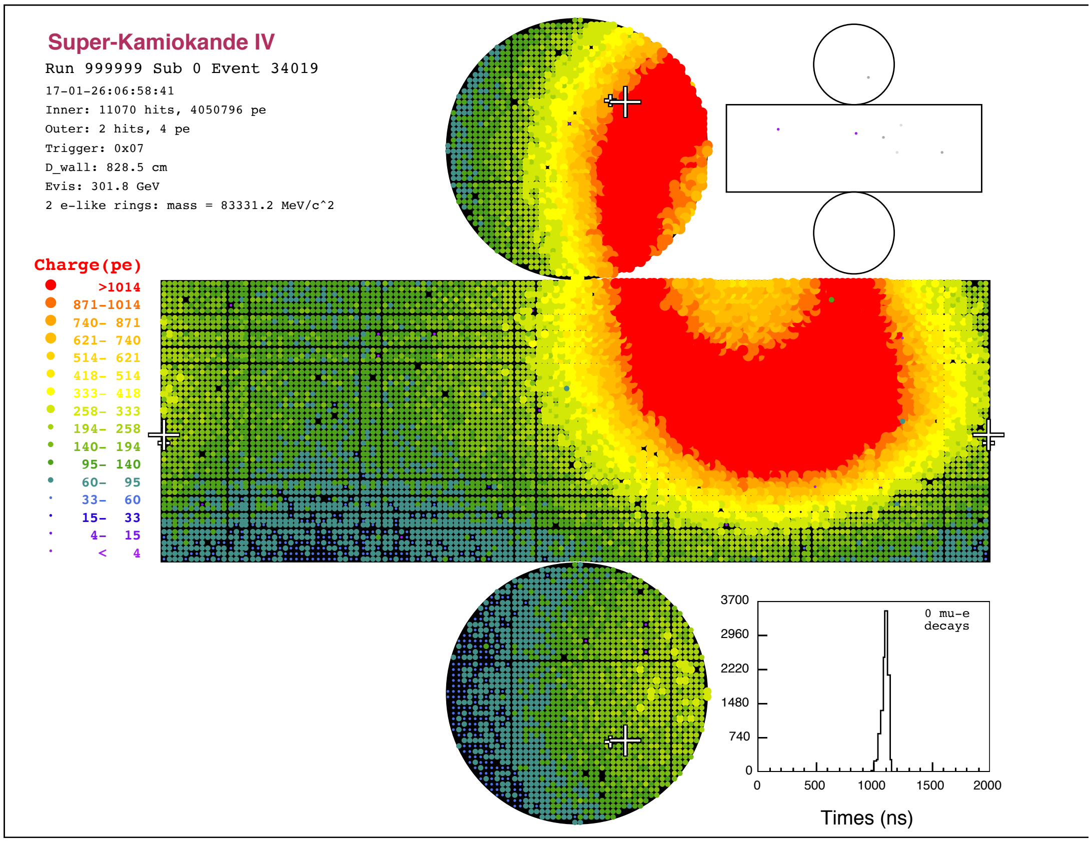


FIG. 3. An example MC event passing all analysis cuts with visible energy of 302 GeV. This event is a simulated 956 GeV electron. Note the charge scale is different from those in Figs. 1 and 2.

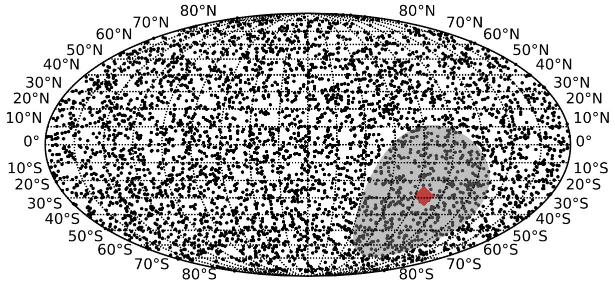


(a)$E_{vis}$ < 1.33 GeV

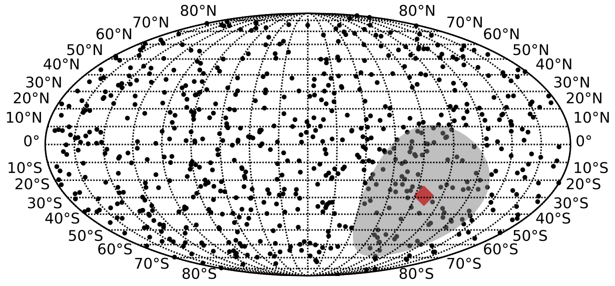


(b)1.33 GeV< $E_{vis}$ < 20 GeV

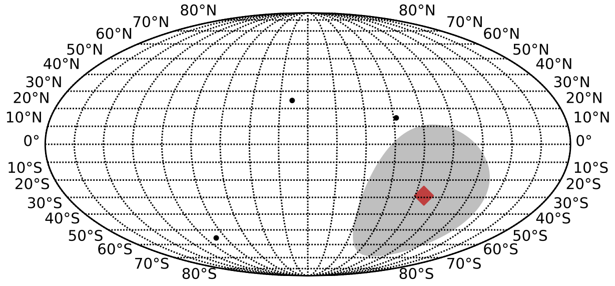


(c)$E_{vis}$ > 20 GeV

FIG. 4. Location of every event passing the analysis cuts in each energy range. The red diamond is the location of the Galactic Center, and the gray region is a 40° cone around the Galactic Center.
